# Supplementary material for: Communication-Efficient Distributed On-Device LLM Inference Over Wireless Networks
Source: arXiv:2503.14882 source file (2025-03-19)
Supplement: Supplementary file 1 [file appendix.tex]

\section*{Appendix}

\subsection{Detailed Neural Network Architecture}
As indicated in Section. \ref{sec:system_model}, we provide the detailed neural network architecture for `ResNet', `ResNet, $\uparrow$ 2', `ResNet $\downarrow$ 2' in Fig. \ref{fig:fig_NN_appendix} (a) and the CA module in Fig. \ref{fig:fig_NN_appendix} (b) which are used in the source. relay and destination nodes. To be specific, the `ResNet' modules adopt CNN layers as the backbone. Inside `ResNet', we adopt the generalized divisive normalization (GDN) layers for modeling densities of image sources \cite{gdn}. The CA modules take both the SNR values and the mean of the features as input and outputs the scaled features by multiplying the original feature with a learned mask.
\figneuralnetappendix

\subsection{Adaptive to Varying Source-to-Relay Channel Conditions} 
As shown in Fig. \ref{fig:fig_SA}, with the CA module, the proposed DeepJSCC schemes are adaptive to varying $\gamma$ values. We further illustrate that the proposed scheme can also adapt to different source-to-relay channel conditions by training with varying $SNR_{sr}$ values. In this experiment, the DeepJSCC-PF model is trained with varying $SNR_{sr} \in [6, 18]$ dB and $\gamma \in [2, 10]$ dB. We then consider training different networks for fixed $SNR_{sr} \in \{8, 10, 12, 14, 16\}$ dB with $\gamma \in [2, 10]$ dB. 

As shown in Fig. \ref{fig:fig_adapt_appendix}, the $SNR_{sr}$ adaptive model together with the models trained at fixed $SNR_{sr}$ values are tested under $\gamma \in \{4, 6\}$ dB. It can be seen that the $SNR_{sr}$ adaptive model achieves comparable performance with the models trained with fixed $SNR_{sr}$ which verifies that the proposed scheme with CA module is effective. 

\figadaptappendix
\figcliffeffect

\subsection{Avoiding the Cliff Effect} 
A key advantage of the DeepJSCC over the conventional schemes is that the neural network is able to provide graceful degradation when the channel quality changes from the estimated one and avoid the cliff effect. We show that the proposed scheme for the cooperative relay channel preserves this property. In this simulation, we adopt the aforementioned DeepJSCC-PF model trained with $SNR_{sr} \in [6, 18], \gamma \in [2, 10]$ dB. We set $SNR_{sr} = 12$ dB and assume the estimated channel quality for $\mathrm{S}-\mathrm{D}$ and $\mathrm{R}-\mathrm{D}$ links are $\gamma_{est} = 6$ dB. The actual channel quality $\gamma_{real}$, however, may be different with $\gamma_{est}$ which is set as $\gamma_{real} \in \{2, 4, 6, 8, 10\}$ dB.

As shown in Fig. \ref{fig:fig_cliff_effect}, we compare the PSNR performance of the `DeepJSCC-PF, $\gamma_{est} = 6$ dB' curve where the channel quality estimation error exists with 
the `DeepJSCC-PF, $\gamma_{est} = \gamma_{real}$' curve where the estimated channel quality always matches the actual channel. The two curves have the same performance at $\gamma_{real} = 6$ dB as the actual SNR and the estimated SNR coincides. We further observe the proposed scheme provides a graceful degradation to the channel estimation error which differs from the digital baseline, which fails when $\gamma_{real}$ is below a certain threshold compared with $\gamma_{est}$.
